# Supplementary material for: Chemical Bonding in Metallic Glasses from Machine Learning and Crystal Orbital Hamilton Population
Source: arXiv:2003.02722 ancillary file (2020-07-21)
Supplement: Supplementary file 1 [file supinfo.pdf]

# Supporting Information for: Chemical Bonding in Metallic Glasses from Machine Learning and Crystal Orbital Hamilton Population

Ary R. Ferreira*

*Department of Physics, Universidade Federal de São Carlos (UFSCar), 13565–905, São Carlos, SP, Brazil*

E-mail: ary.ferreira@df.ufscar.br

## S1 Structural Models

As mentioned in the main text, all the classical molecular dynamics (CMD) simulations were carried out using the velocity-Verlet integrator as implemented in the LAMMPS package[S1] (release 16Feb2016). The embedded atom model (EAM) interatomic potential developed and properly tested by Cheng *et al.*[S2] was used with a cutoff radius of 6.5 Å to describe the interatomic forces in all metallic glasses (MGs). The reader is also referred to the Supplemental Material of Ref. S2, where it is shown that the structure factor simulated with configurations of the MG $Zr_{46}Cu_{47}Al_7$ obtained from CMD simulations match very well with the experimental counterparts; and the same is true for Cu K-edge EXAFS of a Zr-Cu binary alloy. Moreover, this same EAM potential has also been employed in a previous work,[S3] in which theoretical glass transition temperatures have been found to be fairly compatible with experimental counterparts reported by Yokoyama *et al.*,[S4] for a series of Zr-Cu-Al alloys. In addition to that information regarding validation, it is important to remark that this

EAM potential has been widely used for years; providing valuable theoretical support to experimental studies until recently.[S5,S6] In fact, it is known that the transferability of the referred EAM potential can be improved; in order to provide a better overall description of short-range order over a fully range of nominal compositions of the Zr-Cu-Al alloy.[S7] However, it is certainly appropriate for the goals of the present study.

The statistical equivalence between the ensemble of 100-atoms cells of each NC and the respective 10000-atoms cell mentioned in the main text was verified by assessing the convergence of chemical environments statistics for the NCs $Zr_{49}Cu_{49}Al_2$ and $Zr_{45}Cu_{45}Al_{10}$. In order to compare chemical environments in the respective cells, the smooth overlap of atomic positions (SOAP)[S8] descriptor – introduced in the main text – was used. The respective SOAP vectors were generated using the QUIP package[S9] with a cutoff of 3.75 Å for the definition of the range of each chemical environment around atoms, including all elements in its composition. This cutoff value was based on partial pair distribution functions that are well-known for the MGs of the Zr–Cu–Al (ZCA) alloy.[S2,S3] The spherical harmonics basis band limit and the number of radial basis functions were set to 6 and 8, respectively. All the remaining parameters were set with their default values. The referred equivalence was verified and depicted as histograms in Figs. S1 to S12, whose captions are self-explanatory.

As pointed out in the main text, some of the 100-atoms cells listed in Table 1 of the main text were submitted to density functional theory (DFT)[S10,S11] first-principles calculations to set up the databases of interactions (DBIs) required to train the machine learning (ML) model. Regarding the assumed transferability among DBIs of different NCs mentioned in the main text, it has been evidenced from the good results obtained for the Gaussian process regressions (GPRs) made for Al–Al interactions in the DBIs of the NCs $Zr_{49}Cu_{49}Al_2$ and $Zr_{47}Cu_{47}Al_6$. As shown in Table S1, both GPRs were done using the DBI of the NC $Zr_{45}Cu_{45}Al_{10}$.

# S2 CMD Simulations of Uniaxial Compression

The CMD simulations of the uniaxial compression procedure were carried out firstly with huge 80000-atoms cells; starting from the corresponding 10000-atoms cells generated with the quenching protocol described at the beginning of this section. Although it is well accepted that the referred 10000-atoms cells provide representative statistics regarding static atomic configurations (short- and medium-range orders) in these MGs,[S2] finite size effects on the simulations of the uniaxial compression tests have been checked anyway. Therefore, the 80000-atoms cells were built from the $2{\times}2{\times}2$ propagation of the corresponding 10000-atoms cells. Next, adopting a reduced (rather tight) time step of 1 fs, each MG structure at 300 K was first allowed to relax again, but now in the canonical ($NVT$) ensemble for $\Delta t = 100$ ns (the time evolution of the CMD simulation); and, subsequently, for more $\Delta t = 150$ ns in the micro-canonical ($NVE$) ensemble.

So, after verifying constant temperature in that last time evolution, the cubic cell started to be compressed along $x$ direction at a rate of $1{\times}10^7$ s$^{-1}$ in the $NPT$ ensemble using a barostat controlling only perpendicular pressure dissipation; following the approach mentioned in the main text.[S12] That compression rate was chosen after the convergence test shown in Fig. S31. The experimental true stress was compared with the component of the symmetric pressure tensor parallel to the loading direction. That tensor is composed by kinetic energy and virial contributions as implemented in the LAMMPS code.[S1]

It is shown in Fig. S32 the resulting stress-strain (SS) curves at 300 K from these CMD simulations performed with the corresponding 80000-atoms cells of each NC at a compression rate of $1{\times}10^7$ s$^{-1}$. The usage of such big cells was justified above with the aim of exploring finite size effects and, as can be seen in Figs. S33 to S36, they do not affect further analyses within the elastic part of the computed SS curves; nor on the onset of plastic deformation.

Furthermore, for the sake of transparency, there is another technical aspect of these CMD simulations that deserves a critical remark here; it refers to the spurious shape of the resulting stress-strain (SS) curves in the portion that corresponds to yield strength (strain $\approx 5\%$) and

further plastic deformation (strain > 5%). The corresponding curves simulated for the MGs of the ZCA alloy are shown in Fig. S32 and, in a word, all bear two common artifactual features that surely have more to do with the approximation used to describe temperature and pressure dissipation introduced above than with the employed EAM potentials – or any other technical aspect of the CMD simulations.

The former artifactual feature is the fact that yield strength is unreasonably pronounced around 5% strain; stressing out that the preceding experimental linear elastic region is fairly reproduced for the aims of the present study. The convergence test made for the compression rate is shown in Fig. S31 and, within the approximation used in this work,[S12] one can see that this specific artifactual feature is very sensitive to that numerical parameter; whose convergence has been reached at $1\times10^7$ $s^{-1}$. Nevertheless, as expected, the region of the SS curves in which stress is proportional to strain is not dependent on the compression rate (see also in Fig. S31), and the predicted elastic moduli are also fairly satisfactory for the purposes of this work (see caption of Fig. S32). Despite that specific mechanical property has been systematically underestimated in the simulations – another artifact of the adopted approach – the associated linear regressions depicted in Fig. S32 made for each NC follow the trends revealed in Ref. S13.

The second artifact observed in the SS curves is the large plasticity predicted for all four NCs; what – as already introduced above – is simply not compatible with the experimental results reported in Ref. S13, in which the MG $Zr_{45}Cu_{45}Al_{10}$ was found to be very brittle. Moreover, localized nanocrystallization within shear bands and its relationship with the extended plasticity reported for the NC $Zr_{49}Cu_{49}Al_2$ (also in Ref. S13), is certainly not being predicted by the CMD simulations associated to the SS curves shown in Fig. S32; simply because the employed structural models do not accommodate such microstructural aspects. Moreover, it is well-known that enhanced plasticity at room-temperature is a common feature of MG matrix composites of the ZCA alloy system,[S14–S16] whose microstructure is heterogeneous and composed by nanocrystals of concurrent phases immersed in the amorphous

matrix.

The solution could be to increase the structural models up to some dozens (or even few hundreds) of millions of atoms; or, in a much more consistent approach, resort to a multiscale-based strategy. For instance, one could derive an upscaled peridynamic model to describe the brittle behavior of the MG $Zr_{45}Cu_{45}Al_{10}$; or parameterize a constitutive model to describe the SS curve of the MG $Zr_{49}Cu_{49}Al_2$ accounting for localized nanocrystallization. However, this is definitely out of the scope of the present work and unnecessary for its aims. As well commented in the Supporting Information, the elastic portions of the SS curves and respective onset of plastic deformation (strain $\lessapprox$ 5%) are fairly reproduced and consistent with the experiments reported in Ref. S13.

Lastly, also noteworthy is the effect of Zr-content on the chemistry of the MGs of the ZCA alloy. Fig. S54 provides an analog of Fig. 3 of the main text for three additional NCs, namely: $Zr_{40}Cu_{54}Al_6$, $Zr_{47}Cu_{46}Al_7$, and $Zr_{51}Cu_{39.5}Al_{9.5}$. From which one can see that, as could be expected, the overall shapes of the distributions are virtually the same, i.e., the bond strength profile of that alloy does not depend on the NC. Naturally, the fractions of individual distributions are the only feature that depends on the NC.

# S3 Tables and Figures

Table S1: Statistics from a set of equivalent Gaussian process regressions (GPRs) made using the databases listed in Table 1 of the main text. Are listed: (in eV) variances (var.), standard deviations (std.), root-mean-square errors (RMSE), and the maximum -ICOHP value predicted (max.). ML parameters set for most interaction types are: $\theta = 0.5$, with exception of Zr–Cu ($\theta = 1.0$); $\gamma = 0.010$, with exception of Cu–Al ($\gamma = 0.005$) and Zr–Cu ($\gamma = 0.040$). For most GPRs, the training set size (TrSS) was 2000 and the testing set size (TsSS) was 1000 (see exceptions in the footnotes).

| | training set | | testing set | | | |
|---|---|---|---|---|---|---|
| | var. | std. | var. | std. | RMSE | max. |
| $Zr_{45}Cu_{45}Al_{10}$ | | | | | | |
| Al–Al[a] | 0.939 | 0.969 | 0.929 | 0.964 | 0.074 | 4.5 |
| Cu–Al | 0.639 | 0.800 | 0.692 | 0.832 | 0.074 | 4.6 |
| Cu–Cu | 0.143 | 0.379 | 0.141 | 0.375 | 0.078 | 2.5 |
| Zr–Al | 0.871 | 0.933 | 0.926 | 0.962 | 0.091 | 7.7 |
| Zr–Cu | 0.461 | 0.679 | 0.463 | 0.681 | 0.129 | 5.5 |
| Zr–Zr | 1.407 | 1.186 | 1.671 | 1.293 | 0.165 | 15.2 |
| $Zr_{47}Cu_{47}Al_6$ | | | | | | |
| Al–Al[b,c] | 0.854 | 0.924 | 0.611 | 0.781 | 0.084 | 3.6 |
| Cu–Al[d] | 0.690 | 0.831 | 0.579 | 0.761 | 0.062 | 4.4 |
| Cu–Cu | 0.130 | 0.360 | 0.132 | 0.364 | 0.059 | 2.3 |
| Zr–Al[e] | 0.883 | 0.940 | 0.947 | 0.973 | 0.091 | 6.1 |
| Zr–Cu | 0.524 | 0.724 | 0.483 | 0.695 | 0.107 | 5.2 |
| Zr–Zr | 1.420 | 1.192 | 1.391 | 1.179 | 0.121 | 8.3 |
| $Zr_{49}Cu_{49}Al_2$ | | | | | | |
| Al–Al[c,f] | 0.951 | 0.975 | 0.289 | 0.538 | 0.085 | 3.0 |
| Cu–Al | 0.635 | 0.797 | 0.644 | 0.802 | 0.057 | 4.8 |
| Cu–Cu | 0.128 | 0.358 | 0.140 | 0.374 | 0.050 | 2.5 |
| Zr–Al | 0.775 | 0.880 | 0.820 | 0.906 | 0.074 | 6.8 |
| Zr–Cu | 0.484 | 0.695 | 0.460 | 0.678 | 0.084 | 5.2 |
| Zr–Zr | 1.304 | 1.142 | 1.451 | 1.205 | 0.090 | 9.9 |

[a] TrSS = 300; TsSS = 252. [b] TrSS = 300; TsSS = 64.
[c] ML trained with the $Zr_{45}Cu_{45}Al_{10}$ DBI. [d] TrSS = 775.
[e] TrSS = 1497. [f] TrSS = 300; TsSS = 27.

Table S2: Root-mean-square errors (RMSE, in eV) calculated from different Gaussian process regressions made for the nominal composition $Zr_{47}Cu_{47}Al_6$ with distinct training and testing sets sizes.

| testing set size fixed to 1000 | | | |
|---|---|---|---|
| training set size | Cu–Cu | Zr–Cu | Zr–Zr |
| 1400 | 0.0568 | 0.1121 | 0.1193 |
| 1700 | 0.0589 | 0.1096 | 0.1118 |
| 2000 | 0.0575 | 0.1025 | 0.1197 |
| testing set size fixed to 500 | | | |
| training set size | Cu–Al | Zr–Al | |
| 400 | 0.0722 | 0.1198 | |
| 800 | 0.0604 | 0.1018 | |
| 1200 | 0.0574 | 0.0973 | |
| 1600 | – | 0.0933 | |

Table S3: Root-mean-square errors (RMSE, in eV) calculated from different Gaussian process regressions made for the nominal composition $Zr_{49}Cu_{49}Al_2$ with distinct training set sizes and testing set size fixed to 1000.

| training set size | Cu–Al | Cu–Cu | Zr–Al | Zr–Cu | Zr–Zr |
|---|---|---|---|---|---|
| 1400 | 0.0573 | 0.0441 | 0.0754 | 0.0815 | 0.1012 |
| 1700 | 0.0530 | 0.0467 | 0.0724 | 0.0842 | 0.0985 |
| 2000 | 0.0540 | 0.0480 | 0.0729 | 0.0893 | 0.0904 |

Table S4: Bonding data from the two examples of non-persistent local environments (NPLEs) extracted out of the structural model of the MG $Zr_{45}Cu_{45}Al_{10}$ discussed in the main text. The persistent bonds (NPLEs-PBs) at 12% strain are highlighted in bold.

| Zr-centered NPLE | | | Cu-centered NPLE | | |
|---|---|---|---|---|---|
| neighbour | distance (Å) | -ICOHP (eV) | neighbour | distance (Å) | -ICOHP (eV) |
| Zr | 3.89206 | 0.28559 | Cu | 3.07464 | 0.14491 |
| Cu | 3.30096 | 0.35627 | Cu | 3.32458 | 0.08687 |
| Zr | 4.12593 | 0.06545 | Zr | 3.44275 | 0.19441 |
| **Cu** | **2.82047** | **0.88551** | Zr | 2.76334 | 0.96536 |
| **Cu** | **2.66582** | **1.16593** | Zr | 2.83431 | 0.88721 |
| Al | 2.99121 | 1.74771 | Zr | 2.88604 | 0.76907 |
| **Zr** | **3.30921** | **1.17829** | Zr | 2.65566 | 1.23840 |
| Zr | 3.95504 | 0.19691 | **Zr** | **3.34238** | **0.29210** |
| **Zr** | **3.91596** | **0.24038** | **Al** | **2.42334** | **1.64945** |
| **Cu** | **2.86651** | **0.90395** | **Zr** | **2.81331** | **0.89795** |
| **Cu** | **2.70335** | **1.23265** | **Zr** | **2.80312** | **0.84495** |
| **Cu** | **3.03769** | **0.63102** | | | |
| **Cu** | **3.70933** | **0.14486** | | | |
| **Zr** | **3.12364** | **1.64193** | | | |
| **Cu** | **3.19588** | **0.49020** | | | |
| **Cu** | **2.76409** | **1.07609** | | | |
| **Cu** | **3.46659** | **0.29136** | | | |
| **Cu** | **3.22517** | **0.43420** | | | |
| **Zr** | **3.39321** | **0.94385** | | | |

Table S5: Time evolution over compression of the number of non-persistent local environments (NPLEs, see main text) centered at Zr, Cu, and Al atoms; counted for the two extreme NCs $Zr_{45}Cu_{45}Al_{10}$ and $Zr_{49}Cu_{49}Al_2$.

| | $Zr_{49}Cu_{49}Al_2$ | | | $Zr_{45}Cu_{45}Al_{10}$ | | |
|---|---|---|---|---|---|---|
| strain (%) | Zr | Cu | Al | Zr | Cu | Al |
| 1.0 | 744 | 104 | 5 | 567 | 57 | 20 |
| 1.5 | 737 | 118 | 6 | 591 | 68 | 22 |
| 2.0 | 781 | 128 | 7 | 609 | 97 | 26 |
| 2.5 | 792 | 130 | 9 | 653 | 116 | 34 |
| 3.0 | 969 | 209 | 8 | 738 | 138 | 48 |
| 3.5 | 1103 | 321 | 12 | 832 | 204 | 50 |
| 4.0 | 1134 | 368 | 14 | 867 | 226 | 68 |
| 4.5 | 1274 | 420 | 16 | 1017 | 315 | 84 |
| 5.0 | 1502 | 574 | 23 | 1164 | 373 | 88 |
| 5.5 | 1825 | 794 | 25 | 1396 | 519 | 122 |
| **6.0** | **2017** | **925** | **33** | **1679** | **768** | **177** |
| 6.5 | 2296 | 1177 | 48 | 2081 | 1098 | 259 |
| 7.0 | 2536 | 1427 | 48 | 2363 | 1376 | 304 |
| 7.5 | 2869 | 1799 | 67 | 2550 | 1537 | 337 |
| 8.0 | 3097 | 2027 | 73 | 2753 | 1744 | 393 |
| 8.5 | 3238 | 2223 | 90 | 2947 | 1964 | 429 |
| 9.0 | 3487 | 2531 | 98 | 3063 | 2121 | 439 |
| 9.5 | 3698 | 2763 | 108 | 3140 | 2191 | 466 |
| 10.0 | 3805 | 2955 | 114 | 3309 | 2360 | 500 |
| 10.5 | 3934 | 3038 | 118 | 3475 | 2610 | 557 |
| 11.0 | 4083 | 3226 | 130 | 3589 | 2826 | 613 |
| 11.5 | 4155 | 3373 | 133 | 3670 | 2914 | 619 |
| 12.0 | 4218 | 3442 | 137 | 3727 | 3044 | 658 |

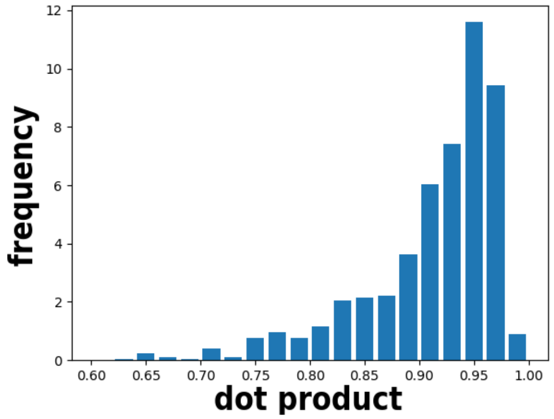


Figure S1: Frequencies of the resulting dot products between the SOAP vector of one Al reference atom and the SOAP vectors of all remaining Al atoms in a 10000-atoms cell of the nominal composition $Zr_{45}Cu_{45}Al_{10}$.

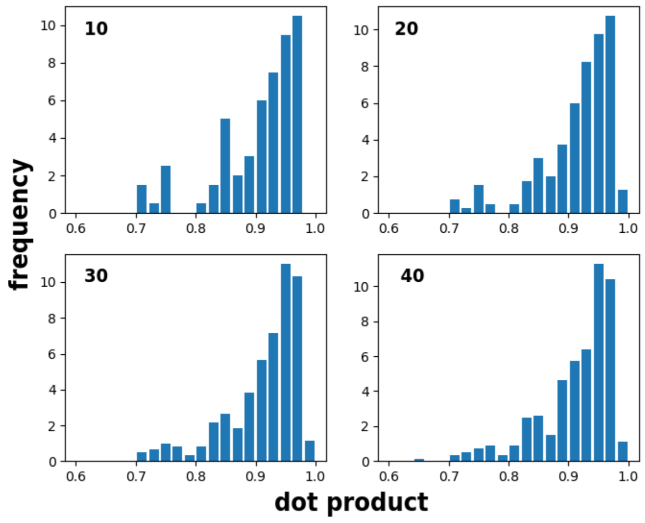


Figure S2: Frequencies of the resulting dot products between the SOAP vector of one Al reference atom taken from a 10000-atoms cell and the SOAP vectors of all Al atoms in different sets of N 100-atoms cells of the nominal composition $Zr_{45}Cu_{45}Al_{10}$. The number N is indicated in each histogram.

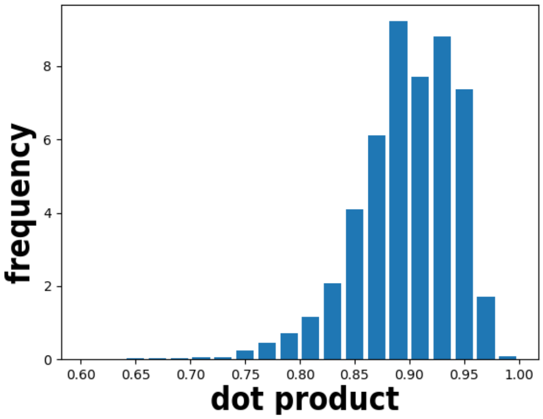


Figure S3: Frequencies of the resulting dot products between the SOAP vector of one Cu reference atom and the SOAP vectors of all remaining Cu atoms in a 10000-atoms cell of the nominal composition $Zr_{45}Cu_{45}Al_{10}$.

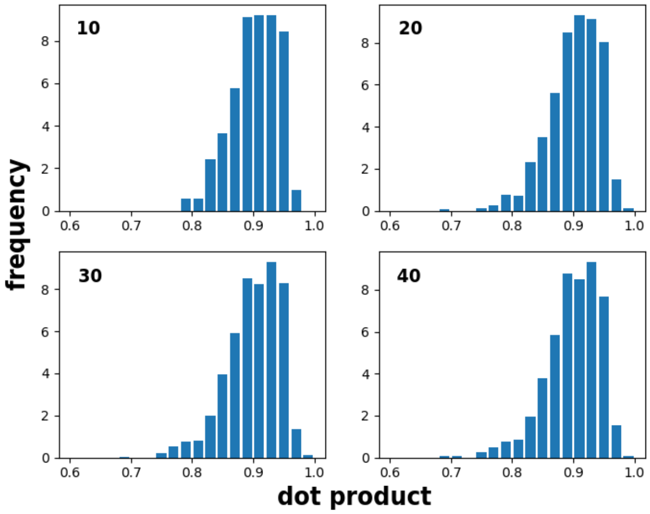


Figure S4: Frequencies of the resulting dot products between the SOAP vector of one Cu reference atom taken from a 10000-atoms cell and the SOAP vectors of all Cu atoms in different sets of N 100-atoms cells of the nominal composition $Zr_{45}Cu_{45}Al_{10}$. The number N is indicated in each histogram.

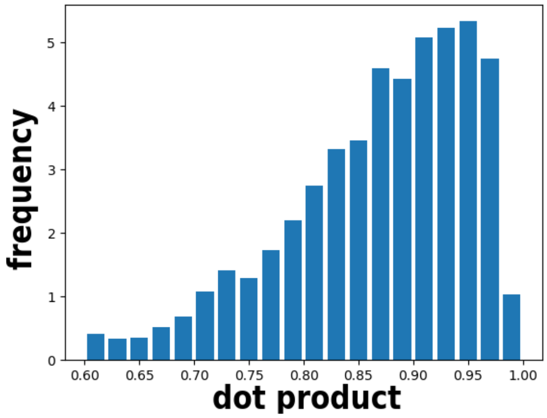


Figure S5: Frequencies of the resulting dot products between the SOAP vector of one Zr reference atom and the SOAP vectors of all remaining Zr atoms in a 10000-atoms cell of the nominal composition $Zr_{45}Cu_{45}Al_{10}$.

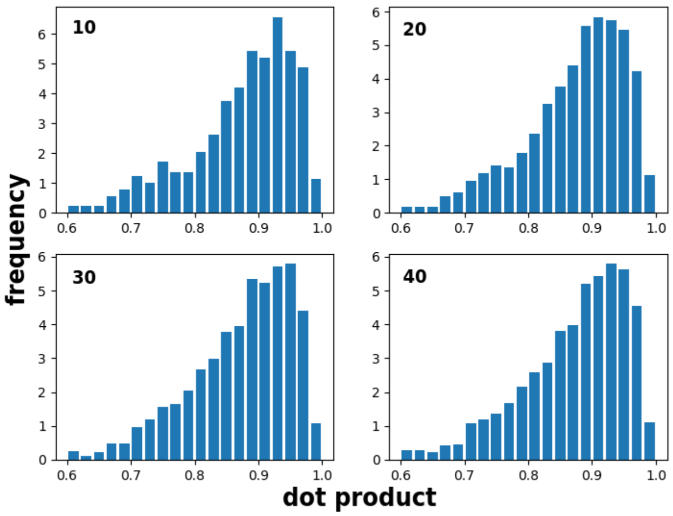


Figure S6: Frequencies of the resulting dot products between the SOAP vector of one Zr reference atom taken from a 10000-atoms cell and the SOAP vectors of all Zr atoms in different sets of N 100-atoms cells of the nominal composition $Zr_{45}Cu_{45}Al_{10}$. The number N is indicated in each histogram.

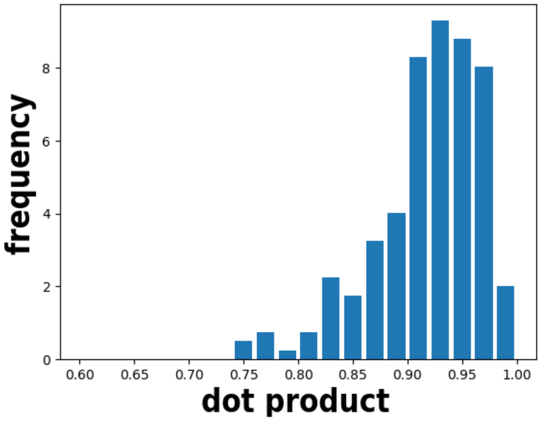


Figure S7: Frequencies of the resulting dot products between the SOAP vector of one Al reference atom and the SOAP vectors of all remaining Al atoms in a 10000-atoms cell of the nominal composition $Zr_{49}Cu_{49}Al_2$.

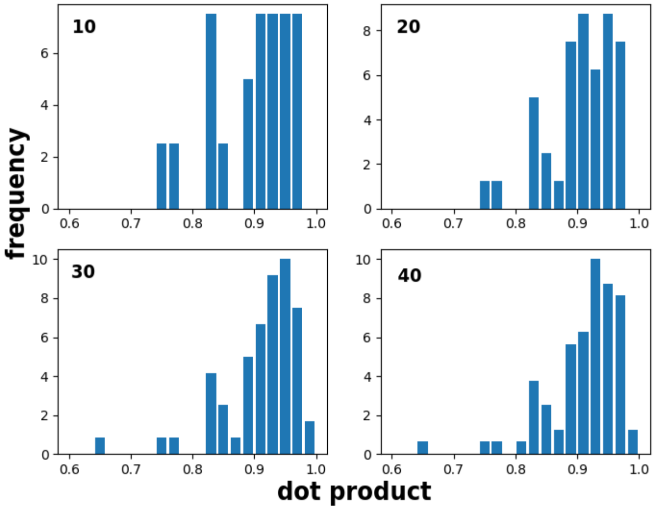


Figure S8: Frequencies of the resulting dot products between the SOAP vector of one Al reference atom taken from a 10000-atoms cell and the SOAP vectors of all Al atoms in different sets of N 100-atoms cells of the nominal composition $Zr_{49}Cu_{49}Al_2$. The number N is indicated in each histogram.

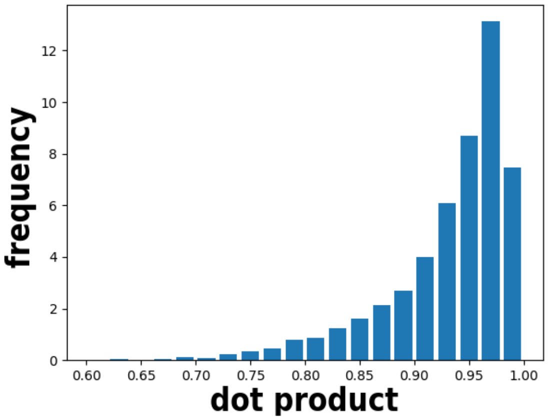


Figure S9: Frequencies of the resulting dot products between the SOAP vector of one Cu reference atom and the SOAP vectors of all remaining Cu atoms in a 10000-atoms cell of the nominal composition $Zr_{49}Cu_{49}Al_2$.

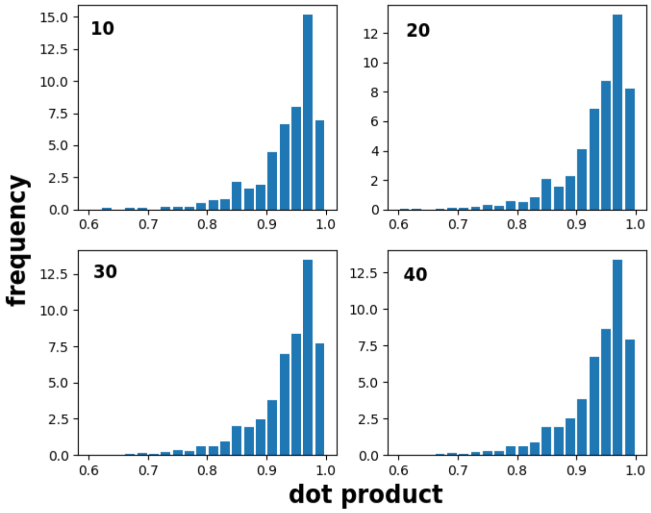


Figure S10: Frequencies of the resulting dot products between the SOAP vector of one Cu reference atom taken from a 10000-atoms cell and the SOAP vectors of all Cu atoms in different sets of N 100-atoms cells of the nominal composition $Zr_{49}Cu_{49}Al_2$. The number N is indicated in each histogram.

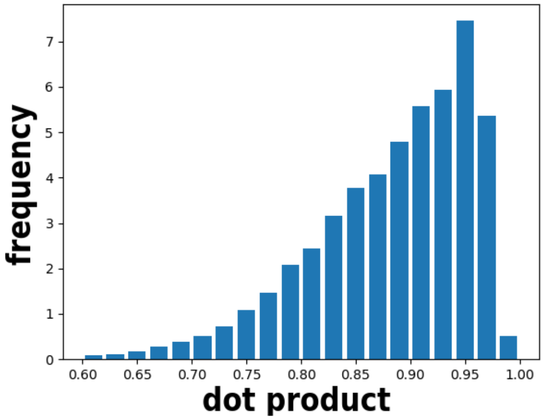


Figure S11: Frequencies of the resulting dot products between the SOAP vector of one Zr reference atom and the SOAP vectors of all remaining Zr atoms in a 10000-atoms cell of the nominal composition $Zr_{49}Cu_{49}Al_2$.

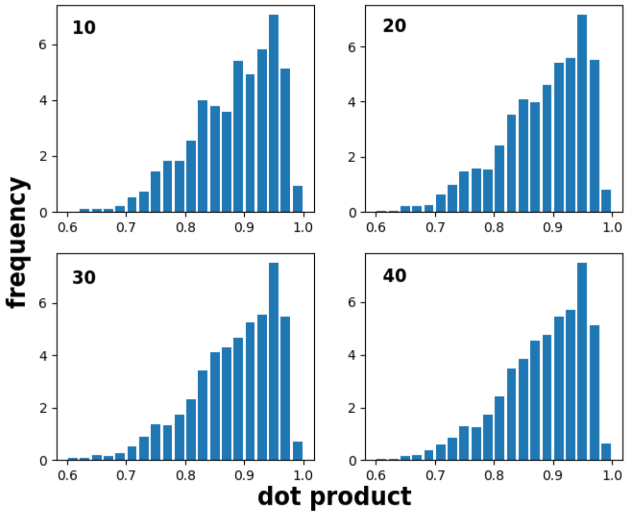


Figure S12: Frequencies of the resulting dot products between the SOAP vector of one Zr reference atom taken from a 10000-atoms cell and the SOAP vectors of all Zr atoms in different sets of N 100-atoms cells of the nominal composition $Zr_{49}Cu_{49}Al_2$. The number N is indicated in each histogram.

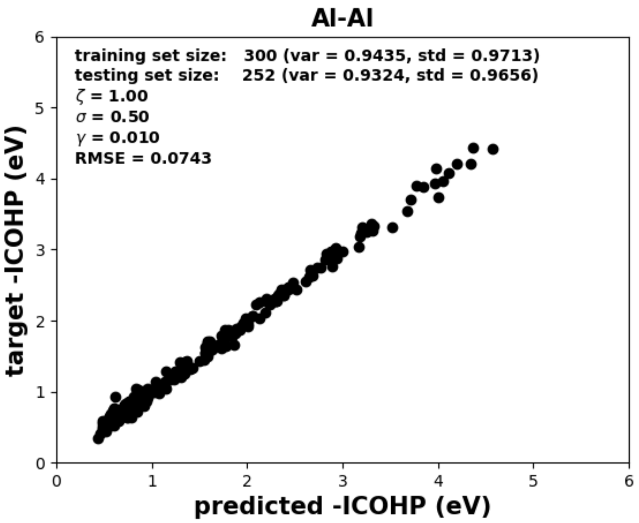


Figure S13: Scatter plot of results from a Gaussian process regression made for the nominal composition $Zr_{45}Cu_{45}Al_{10}$.

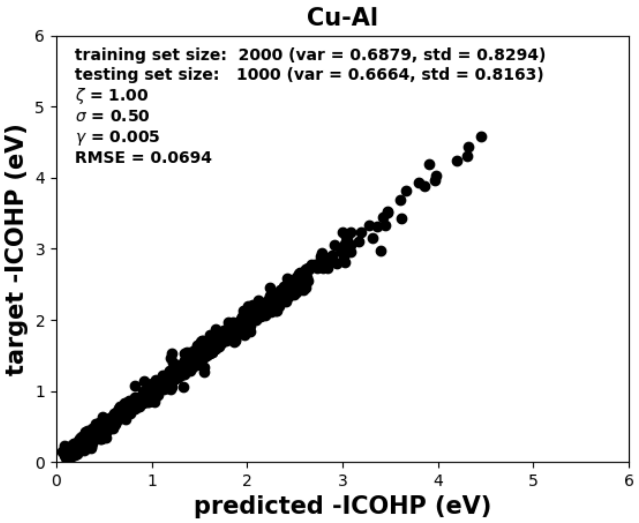


Figure S14: Scatter plot of results from a Gaussian process regression made for the nominal composition $Zr_{45}Cu_{45}Al_{10}$.

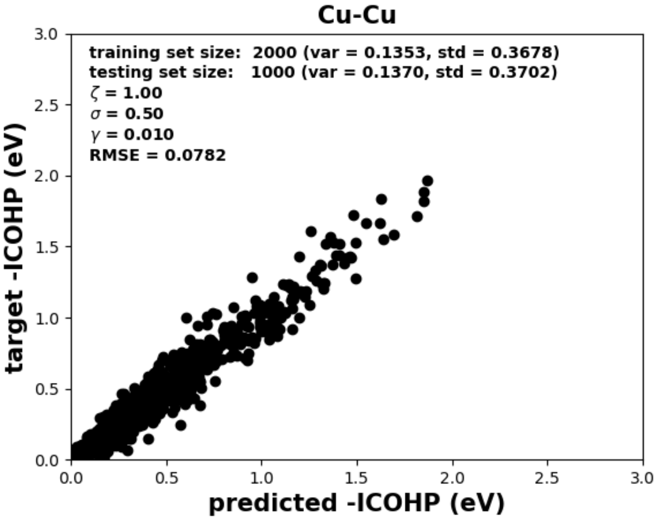


Figure S15: Scatter plot of results from a Gaussian process regression made for the nominal composition $Zr_{45}Cu_{45}Al_{10}$.

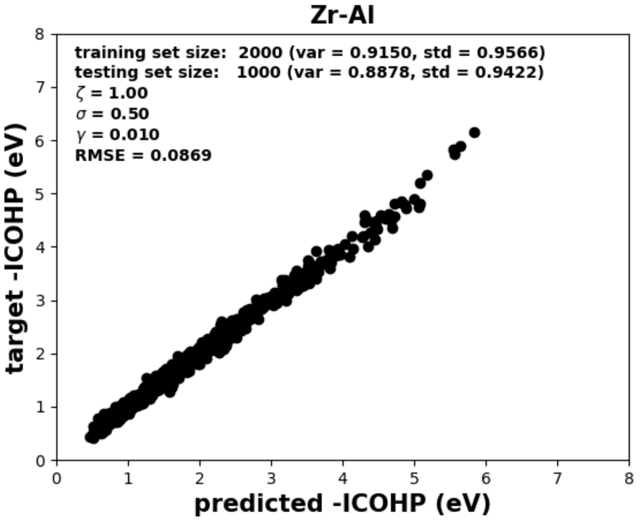


Figure S16: Scatter plot of results from a Gaussian process regression made for the nominal composition $Zr_{45}Cu_{45}Al_{10}$.

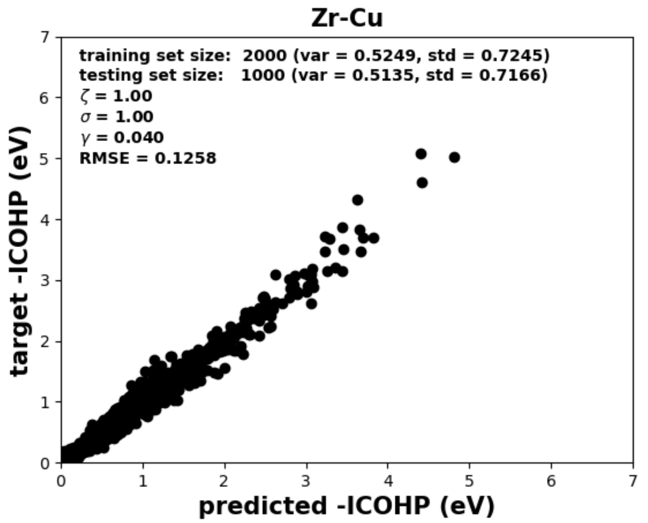


Figure S17: Scatter plot of results from a Gaussian process regression made for the nominal composition $Zr_{45}Cu_{45}Al_{10}$.

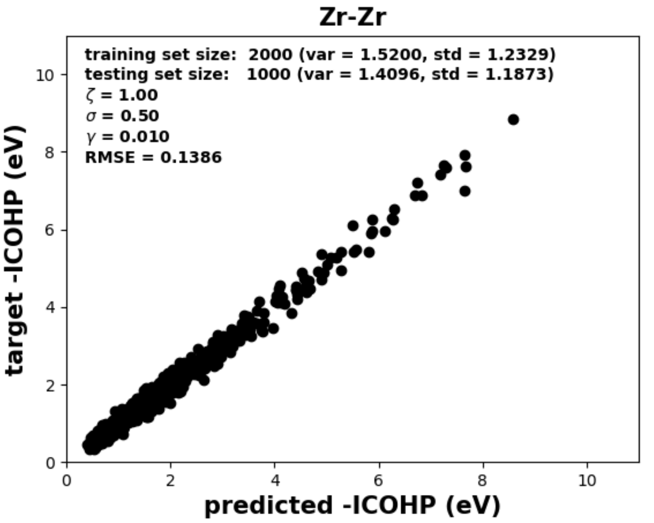


Figure S18: Scatter plot of results from a Gaussian process regression made for the nominal composition $Zr_{45}Cu_{45}Al_{10}$.

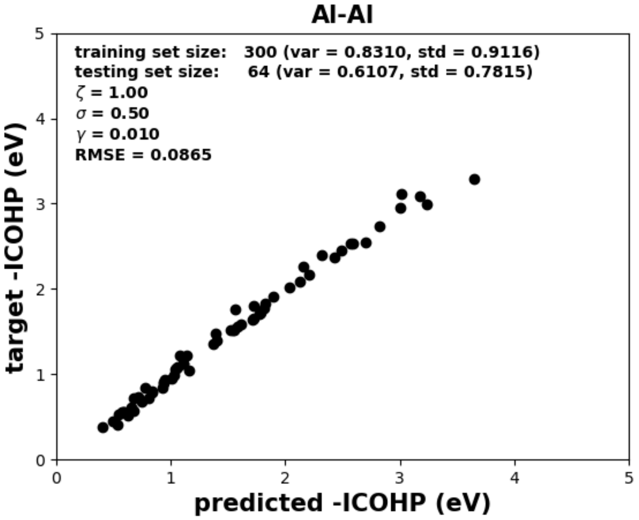


Figure S19: Scatter plot of results from a Gaussian process regression made for the nominal composition $Zr_{47}Cu_{47}Al_6$. In this particular case, the training set database of the nominal composition $Zr_{45}Cu_{45}Al_{10}$ has been used.

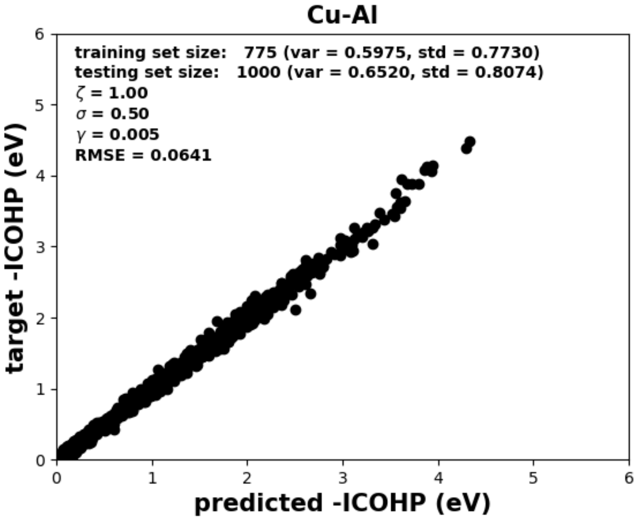


Figure S20: Scatter plot of results from a Gaussian process regression made for the nominal composition $Zr_{47}Cu_{47}Al_6$.

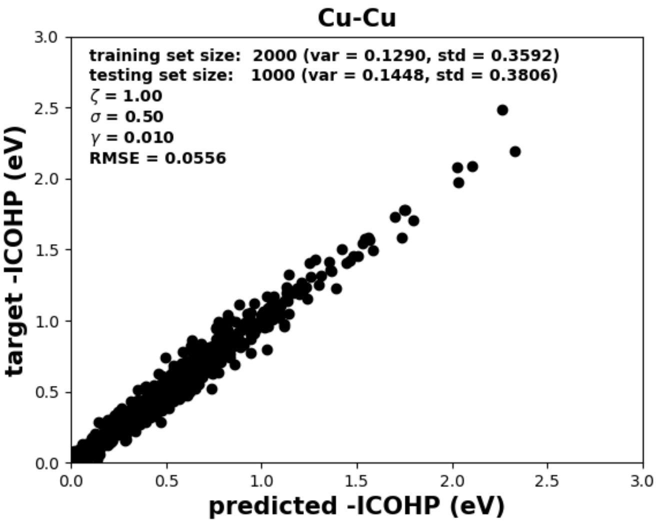


Figure S21: Scatter plot of results from a Gaussian process regression made for the nominal composition $Zr_{47}Cu_{47}Al_6$.

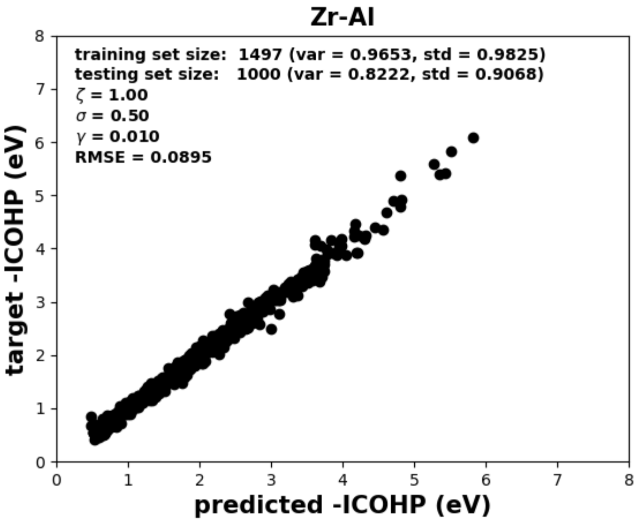


Figure S22: Scatter plot of results from a Gaussian process regression made for the nominal composition $Zr_{47}Cu_{47}Al_6$.

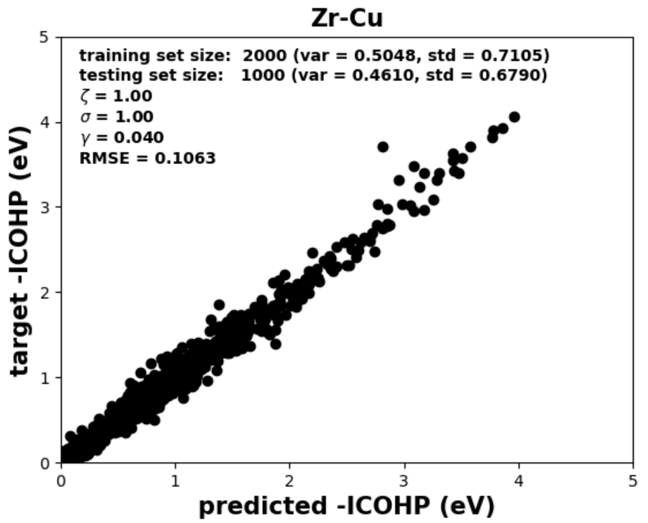


Figure S23: Scatter plot of results from a Gaussian process regression made for the nominal composition $Zr_{47}Cu_{47}Al_6$.

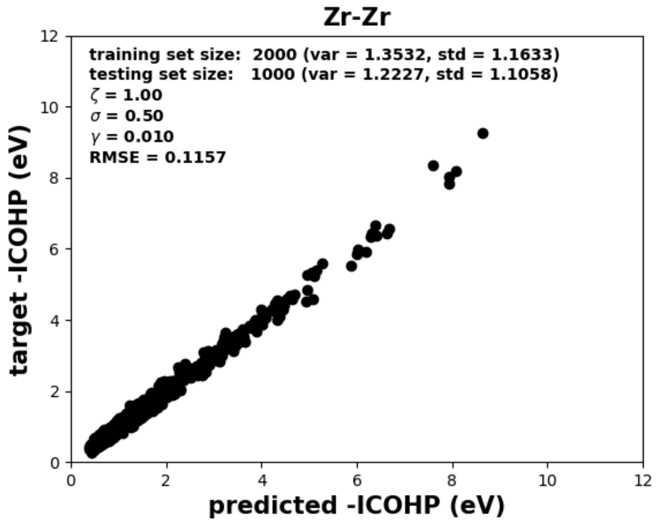


Figure S24: Scatter plot of results from a Gaussian process regression made for the nominal composition $Zr_{47}Cu_{47}Al_6$.

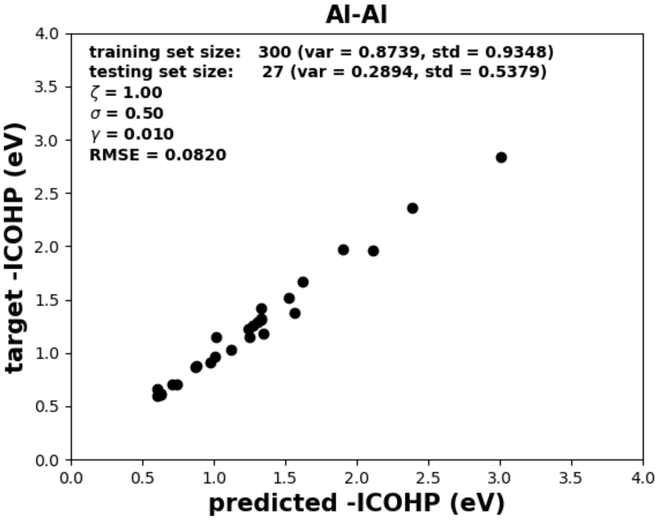


Figure S25: Scatter plot of results from a Gaussian process regression made for the nominal composition $Zr_{49}Cu_{49}Al_2$. In this particular case, the training set database of the nominal composition $Zr_{45}Cu_{45}Al_{10}$ has been used.

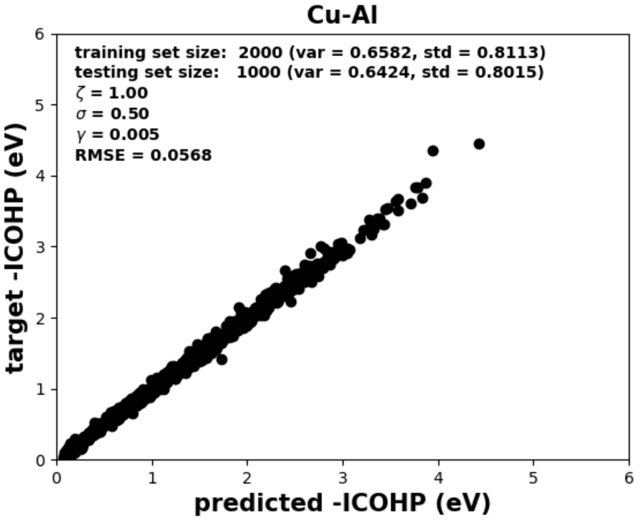


Figure S26: Scatter plot of results from a Gaussian process regression made for the nominal composition $Zr_{49}Cu_{49}Al_2$.

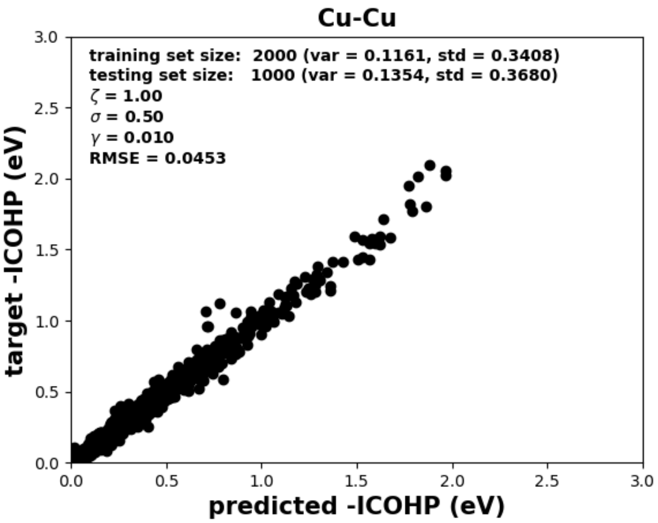


Figure S27: Scatter plot of results from a Gaussian process regression made for the nominal composition $Zr_{49}Cu_{49}Al_2$.

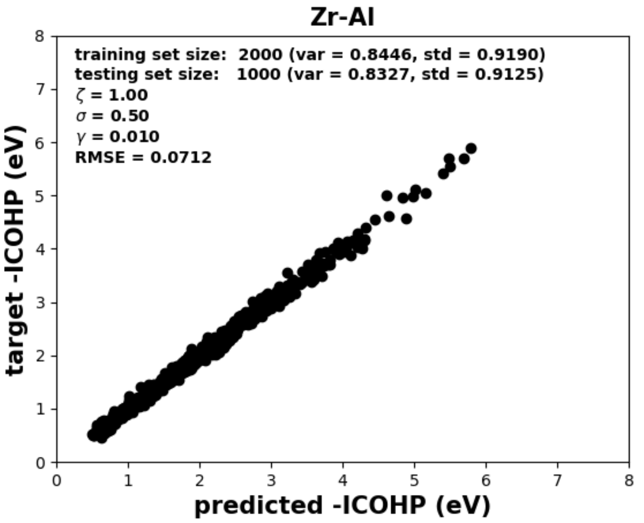


Figure S28: Scatter plot of results from a Gaussian process regression made for the nominal composition $Zr_{49}Cu_{49}Al_2$.

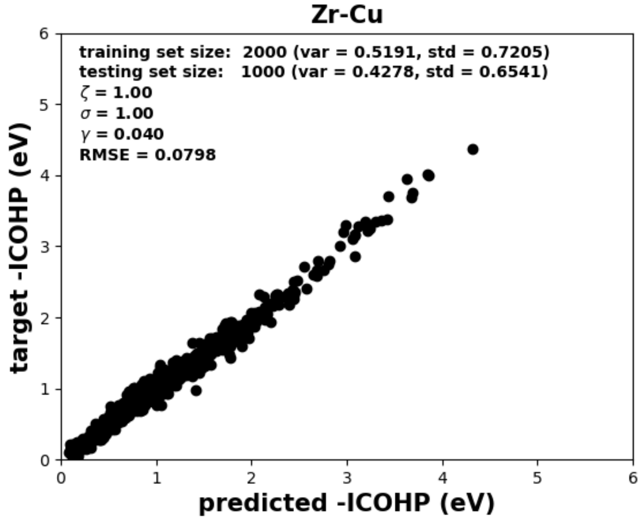


Figure S29: Scatter plot of results from a Gaussian process regression made for the nominal composition $Zr_{49}Cu_{49}Al_2$.

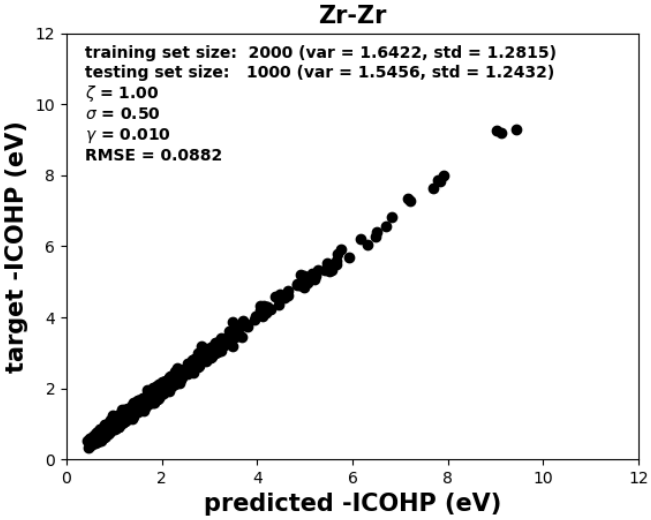


Figure S30: Scatter plot of results from a Gaussian process regression made for the nominal composition $Zr_{49}Cu_{49}Al_2$.

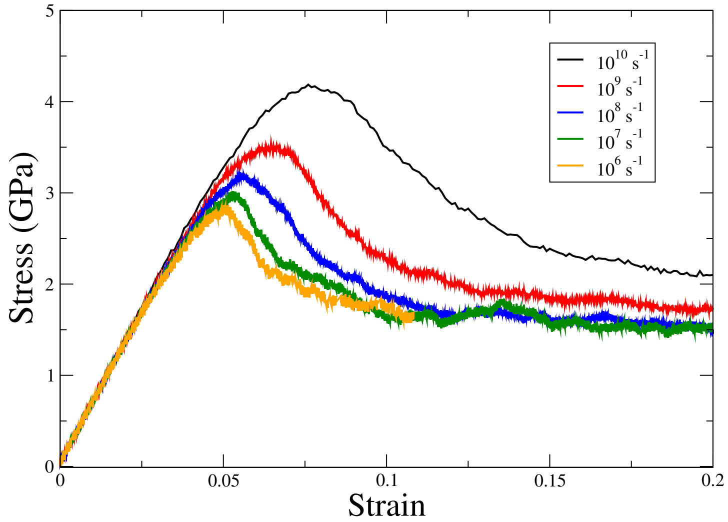


Figure S31: Comparison among the stress-strain curves simulated for 80000-atoms cells of the nominal composition $Zr_{45}Cu_{45}Al_{10}$ at different compression rates.

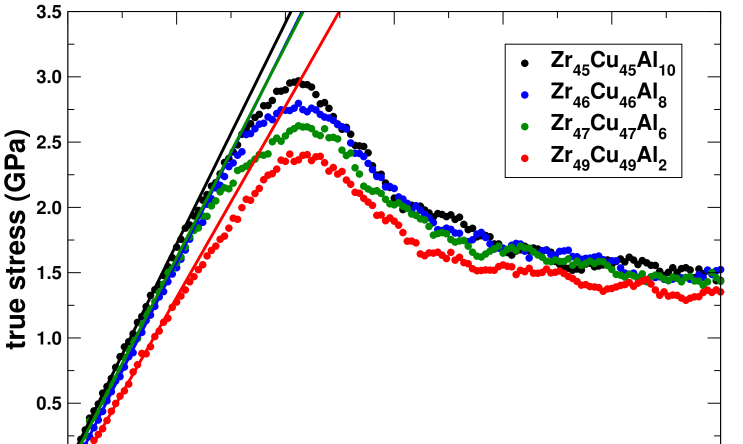


Figure S32: Comparison among the stress-strain curves simulated for 80000-atoms cells at 300 K, with a compression rate of $1\times10^{7}$ s$^{-1}$, for the bulk metallic glasses studied in this work (dotted lines). The resulting respective linear regressions made with points up to 2.5% strain are shown as solid lines, from which it was possible to estimate the respective elastic moduli: $Zr_{45}Cu_{45}Al_{10}$ (67.74 GPa); $Zr_{46}Cu_{46}Al_{8}$ (66.583 GPa); $Zr_{47}Cu_{47}Al_{6}$ (64.867 GPa); and $Zr_{49}Cu_{49}Al_{2}$ (58.602 GPa).

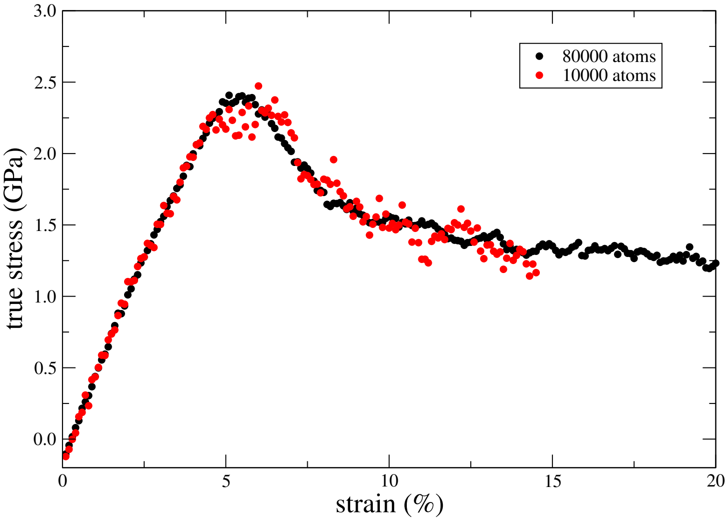


Figure S33: Stress-strain curves simulated for the $Zr_{49}Cu_{49}Al_2$ with different number of atoms and a compression rate of $1{\times}10^7$ $s^{-1}$.

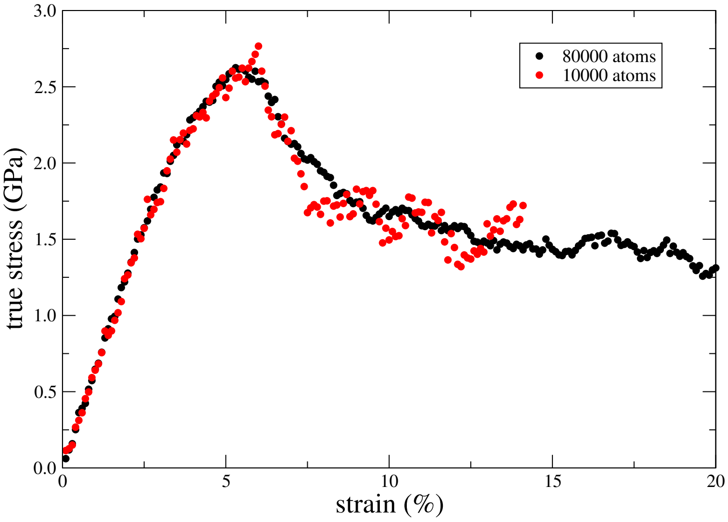


Figure S34: Stress-strain curves simulated for the $Zr_{47}Cu_{47}Al_6$ with different number of atoms and a compression rate of $1{\times}10^7$ $s^{-1}$.

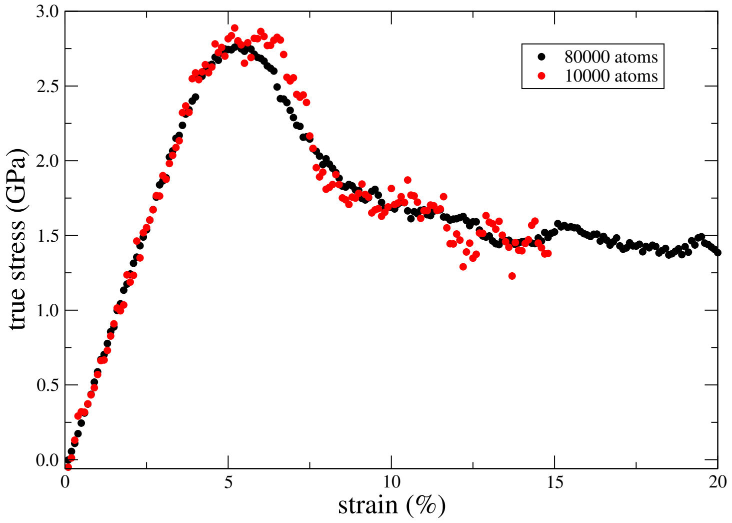


Figure S35: Stress-strain curves simulated for the $Zr_{46}Cu_{46}Al_8$ with different number of atoms and a compression rate of $1{\times}10^7$ $s^{-1}$.

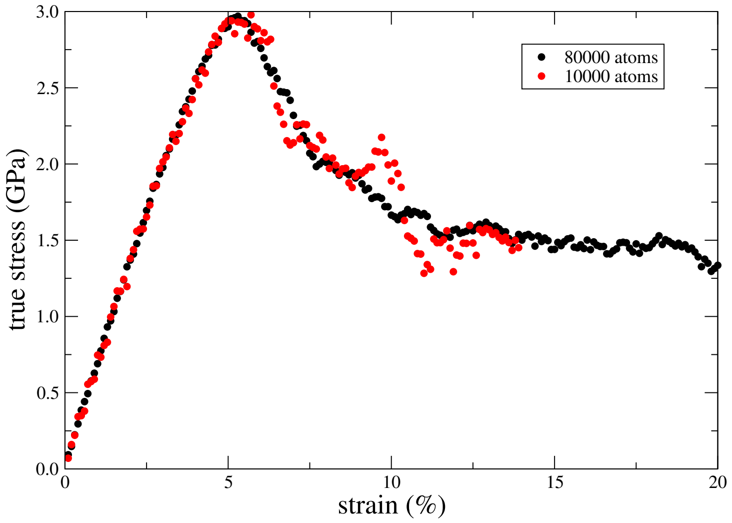


Figure S36: Stress-strain curves simulated for the $Zr_{45}Cu_{45}Al_{10}$ with different number of atoms and a compression rate of $1{\times}10^7$ $s^{-1}$.

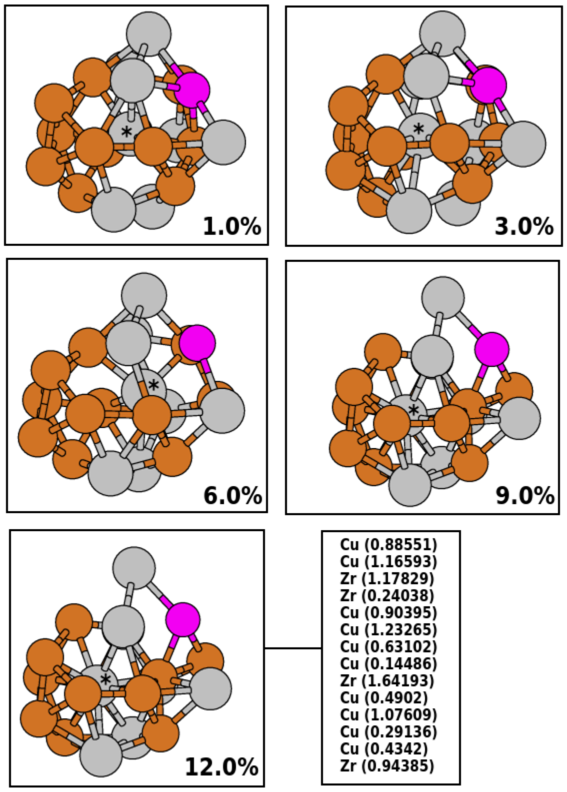


Figure S37: Bonding data and snapshots of the example of non-persistent local environment (NPLE) extracted out of the structural model of the MG $Zr_{45}Cu_{45}Al_{10}$ discussed in the main text.

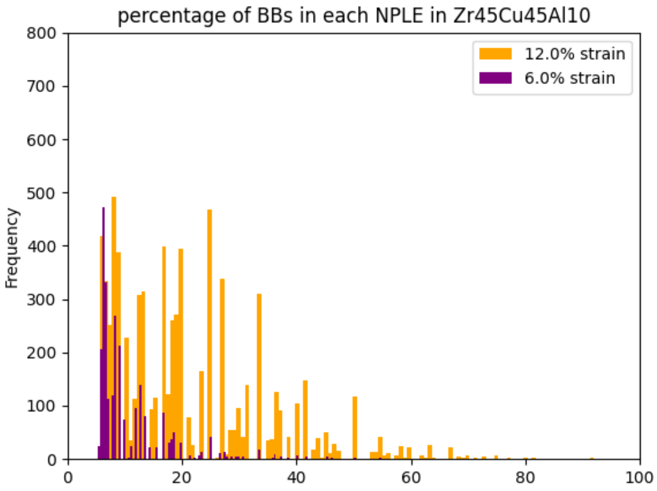


Figure S38: Distributions of percentages of broken bonds (BBs) in individual non-persistent local environments (NPLEs) in the structural model of the MG $Zr_{45}Cu_{45}Al_{10}$. The number of bins in the histogram was calculated from Sturges's formula and arbitrarily multiplied by 10.

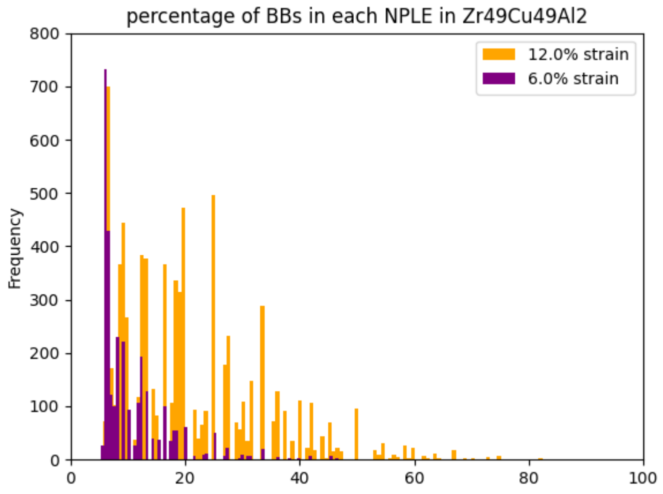


Figure S39: Distributions of percentages of broken bonds (BBs) in individual non-persistent local environments (NPLEs) in the structural model of the MG $Zr_{49}Cu_{49}Al_2$. The number of bins in the histogram was calculated from Sturges's formula and arbitrarily multiplied by 10.

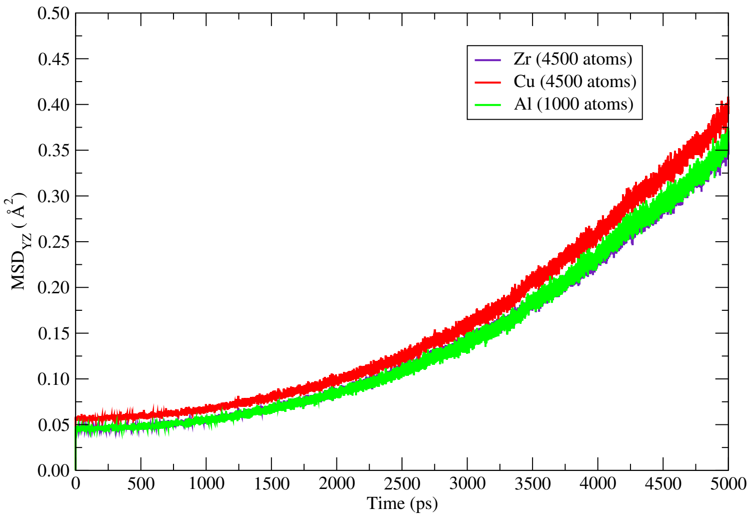


Figure S40: Averaged mean-squared displacements components perpendicular to the loading direction ($MSD_{YZ}$) computed along the uniaxial compression CMD simulations up to 5% strain for the 10000-atoms cells of the MG $Zr_{45}Cu_{45}Al_{10}$. Groups are based on the atomic species.

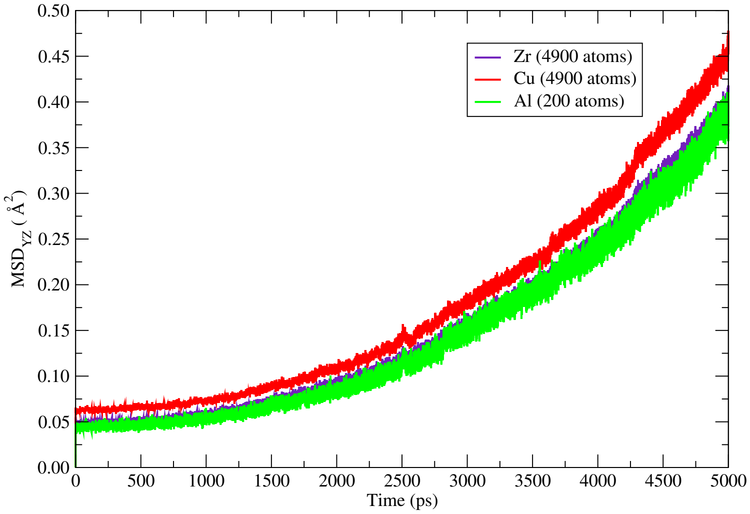


Figure S41: Averaged mean-squared displacements components perpendicular to the loading direction ($MSD_{YZ}$) computed along the uniaxial compression CMD simulations up to 5% strain for the 10000-atoms cells of the MG $Zr_{49}Cu_{49}Al_2$. Groups are based on the atomic species.

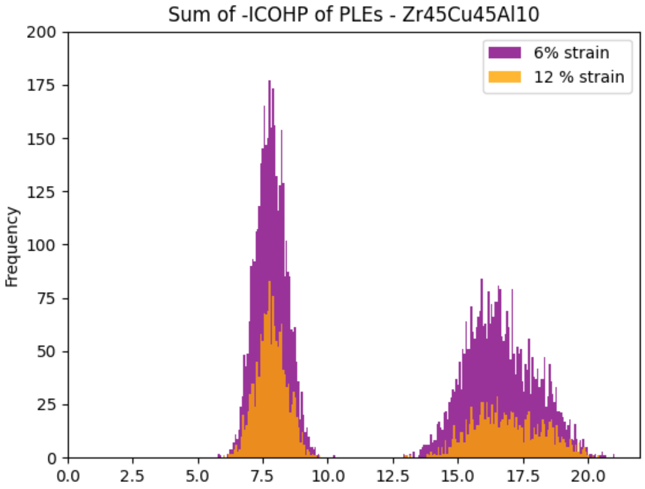


Figure S42: Distributions of the sums of -ICOHP values of persistent bonds (PBs) in persistent local environments (PLEs) in the structural model of the MG $Zr_{45}Cu_{45}Al_{10}$. The number of bins in each histogram was calculated from Sturges's formula and arbitrarily multiplied by 10.

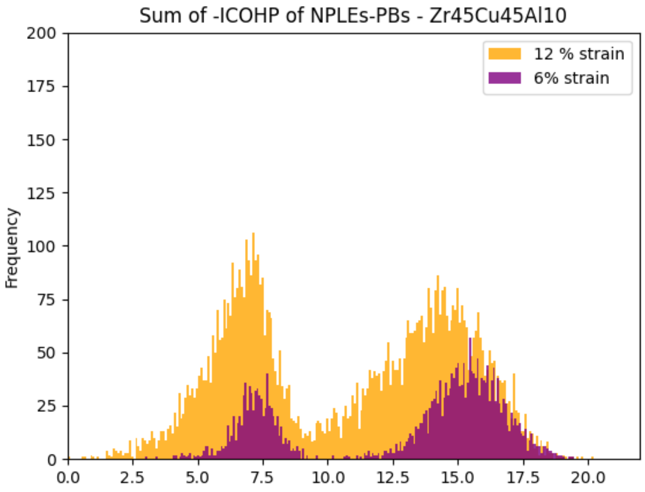


Figure S43: Distributions of the sums of -ICOHP values of persistent bonds (PBs) in non-persistent local environments (NPLEs) in the structural model of the MG $Zr_{45}Cu_{45}Al_{10}$. The number of bins in each histogram was calculated from Sturges's formula and arbitrarily multiplied by 10.

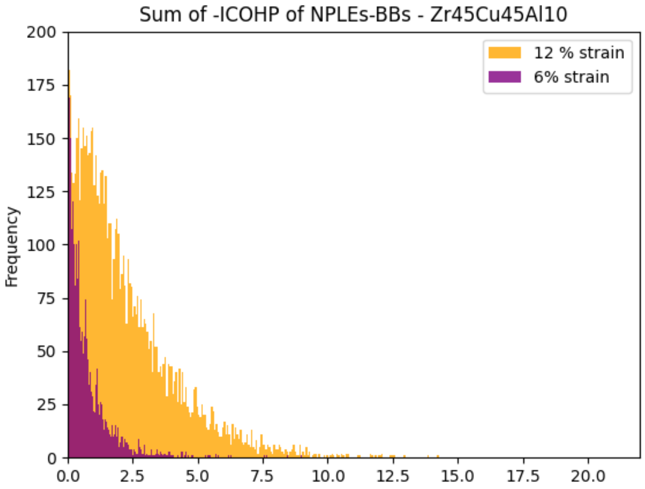


Figure S44: Distributions of the sums of -ICOHP values of broken bonds (BBs) in non-persistent local environments (NPLEs) in the structural model of the MG $Zr_{45}Cu_{45}Al_{10}$. The number of bins in each histogram was calculated from Sturges's formula and arbitrarily multiplied by 10.

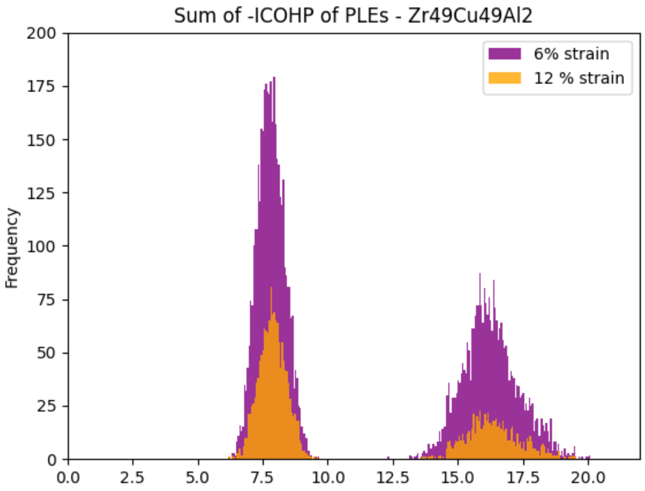


Figure S45: Distributions of the sums of -ICOHP values of persistent bonds (PBs) in persistent local environments (PLEs) in the structural model of the MG $Zr_{49}Cu_{49}Al_2$. The number of bins in each histogram was calculated from Sturges's formula and arbitrarily multiplied by 10.

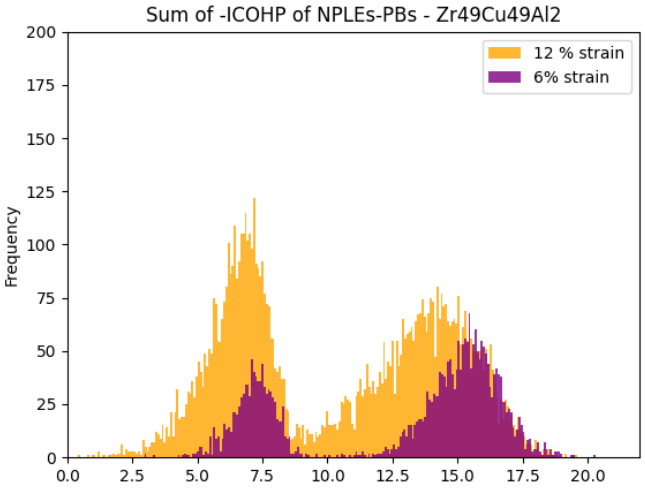


Figure S46: Distributions of the sums of -ICOHP values of persistent bonds (PBs) in non-persistent local environments (NPLEs) in the structural model of the MG $Zr_{49}Cu_{49}Al_2$. The number of bins in each histogram was calculated from Sturges's formula and arbitrarily multiplied by 10.

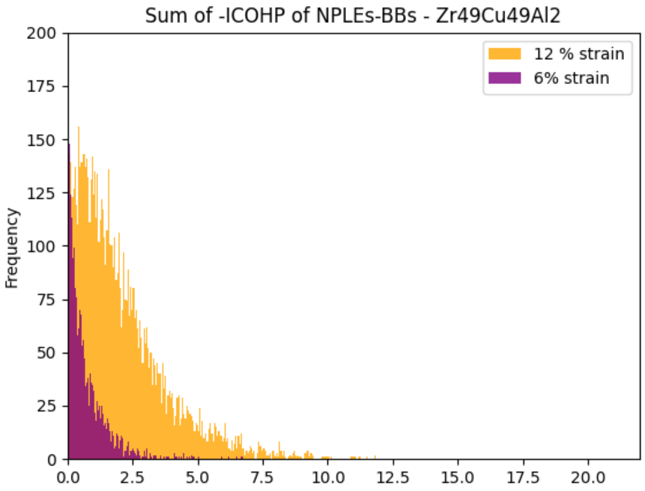


Figure S47: Distributions of the sums of -ICOHP values of broken bonds (BBs) in non-persistent local environments (NPLEs) in the structural model of the MG $Zr_{49}Cu_{49}Al_2$. The number of bins in each histogram was calculated from Sturges's formula and arbitrarily multiplied by 10.

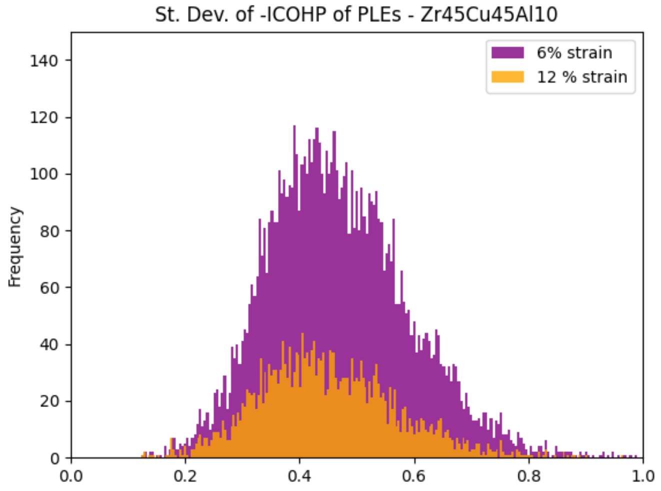


Figure S48: Distributions of the standard deviations of -ICOHP values of persistent bonds (PBs) in persistent local environments (PLEs) in the structural model of the MG $Zr_{45}Cu_{45}Al_{10}$. The number of bins in each histogram was calculated from Sturges's formula and arbitrarily multiplied by 10.

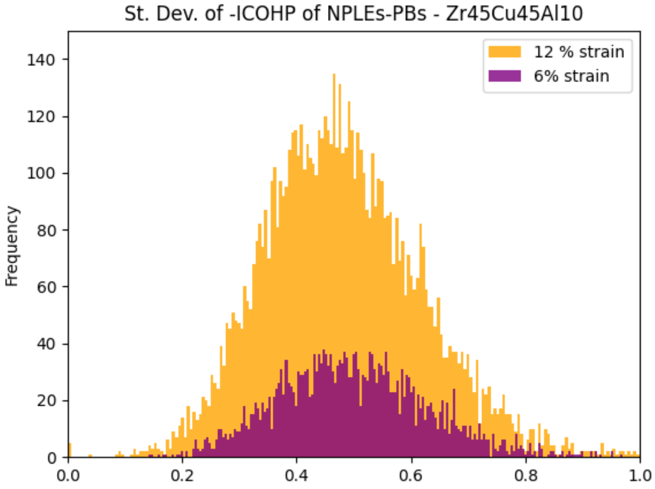


Figure S49: Distributions of the standard deviations of -ICOHP values of persistent bonds (PBs) in non-persistent local environments (NPLEs) in the structural model of the MG $Zr_{45}Cu_{45}Al_{10}$. The number of bins in each histogram was calculated from Sturges's formula and arbitrarily multiplied by 10.

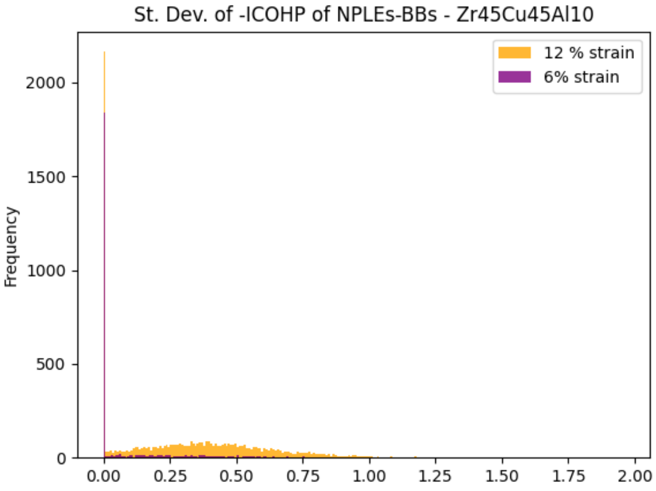


Figure S50: Distributions of the standard deviations of -ICOHP values of broken bonds (BBs) in non-persistent local environments (NPLEs) in the structural model of the MG $Zr_{45}Cu_{45}Al_{10}$. The number of bins in each histogram was calculated from Sturges's formula and arbitrarily multiplied by 10.

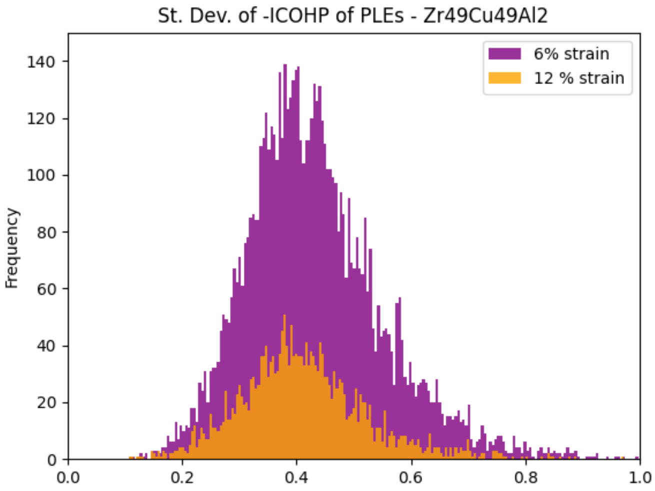


Figure S51: Distributions of the standard deviations of -ICOHP values of persistent bonds (PBs) in persistent local environments (PLEs) in the structural model of the MG $Zr_{49}Cu_{49}Al_2$. The number of bins in each histogram was calculated from Sturges's formula and arbitrarily multiplied by 10.

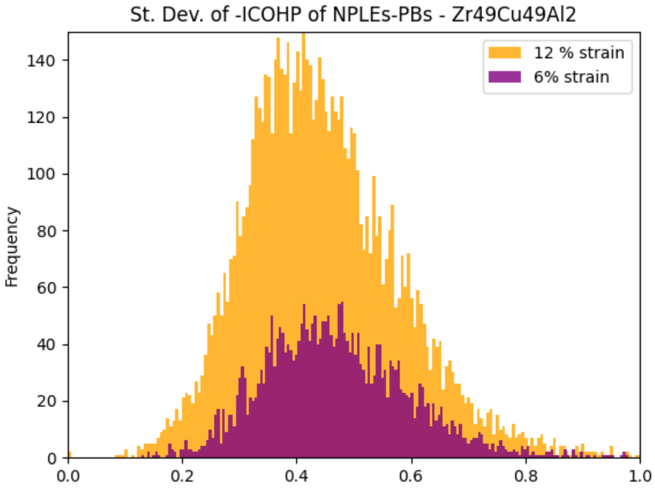


Figure S52: Distributions of the standard deviations of -ICOHP values of persistent bonds (PBs) in non-persistent local environments (NPLEs) in the structural model of the MG $Zr_{49}Cu_{49}Al_2$. The number of bins in each histogram was calculated from Sturges's formula and arbitrarily multiplied by 10.

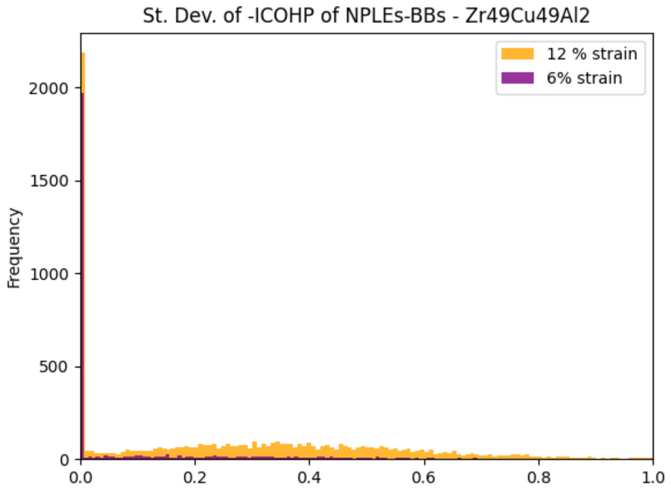


Figure S53: Distributions of the standard deviations of -ICOHP values of broken bonds (BBs) in non-persistent local environments (NPLEs) in the structural model of the MG $Zr_{49}Cu_{49}Al_2$. The number of bins in each histogram was calculated from Sturges's formula and arbitrarily multiplied by 10.

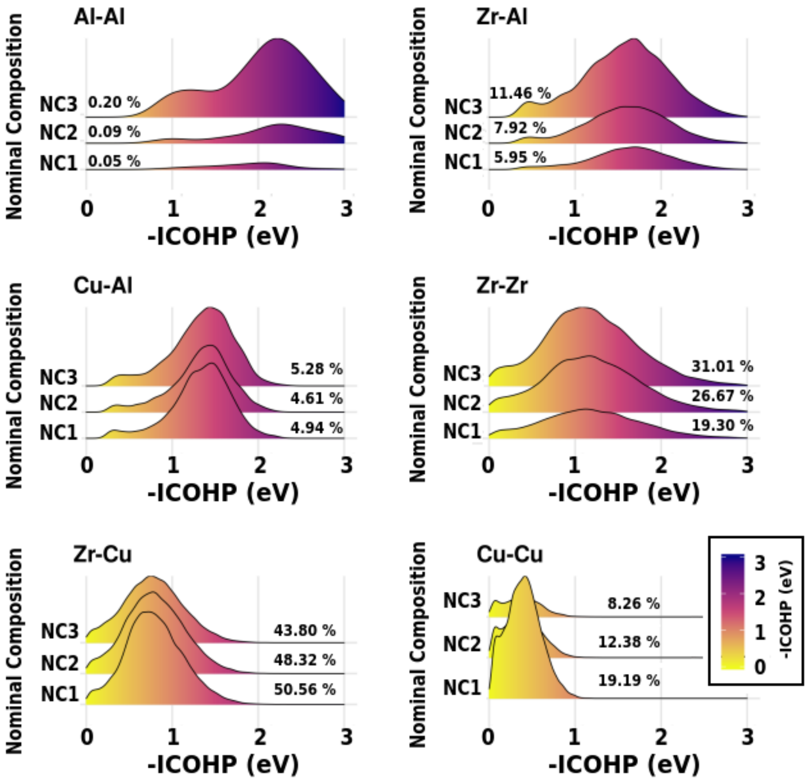


Figure S54: Distributions of -ICOHP values predicted by the ML model for all interatomic interactions existing in 10000-atoms cells of the bulk metallic glasses with nominal compositions $Zr_{40}Cu_{54}Al_6$ (NC1), $Zr_{47}Cu_{46}Al_7$ (NC2), and $Zr_{51}Cu_{39.5}Al_{9.5}$ (NC3). The fractions of each type of interaction are indicated as percentages.

# References

[S1] Plimpton, S. Fast Parallel Algorithms for Short-Range Molecular Dynamics. *J. Comp. Phys.* **1995**, *117*, 1–19.

[S2] Cheng, Y. Q.; Ma, E.; Sheng, H. W. Atomic Level Structure in Multicomponent Bulk Metallic Glass. *Phys. Rev. Lett.* **2009**, *102*, 245501.

[S3] Ferreira, A. R.; Rino, J. P. On the use of atomistic simulations to aid bulk metallic glasses structural elucidation with solid-state NMR. *Scientific Reports* **2017**, *7*, 9305.

[S4] Yokoyama, Y.; Yamasaki, T.; Liaw, P. K.; Inoue, A. Relations between the Thermal and Mechanical Properties of Cast Zr-TM-Al (TM: Cu, Ni, or Co) Bulk Glassy Alloys. *Materials Transactions* **2007**, *48*, 1846–1849.

[S5] Wang, X. H.; Inoue, A.; Zhao, J. F.; Kongc, F. L.; Zhu, S. L.; Kaban, I.; Stoica, M.; Oswald, S.; Fan, C.; Shalaan, E.; Al-Marzouki, F.; Eckert, J.; Yin, F. X.; Li, Q. Liquid ejection temperature dependence of structure and glass transition behavior for rapidly solidified Zr-Al-M (M=Ni, Cu or Co) ternary glassy alloys. *J. Alloys Compd.* **2018**, *739*, 1104–1114.

[S6] Pekin, T. C.; Ding, J.; Gammer, C.; Ozdol, B.; Ophus, C.; Asta, M.; Ritchie, R. O.; Minor, A. M. Direct measurement of nanostructural changeduring in situ deformation of a bulk metallic glass. *Nature Mater.* **2019**, *10*, 2445.

[S7] Kaban, I.; Jóvári, P.; Escher, B.; Tran, D. T.; Svensson, G.; Webb, M. A.; Regier, T. Z.; Kokotin, V.; Beuneu, B.; Gemming, T.; Eckert, J. Atomic structure and formation of CuZrAl bulk metallic glasses and composites. *Acta Materialia* **2015**, *100*, 369–376.

[S8] Bartók, A. P.; Kondor, R.; Csányi, G. On representing chemical environments. *Phys. Rev. B* **2013**, *87*, 184115.

[S9] libAtoms/QUIP molecular dynamics framework. http://www.libatoms.org, Accessed: 2020-07-21.

[S10] Hohenberg, P.; Kohn, W. Inhomogeneous Electron Gas. *Phys. Rev.* **1964**, *136*, B864–B871.

[S11] Kohn, W.; Sham, L. J. Self-Consistent Equations Including Exchange and Correlation Effects. *Phys. Rev.* **1965**, *140*, A1133–A1138.

[S12] Melchionna, S.; Ciccotti, G.; Holian, B. L. Hoover NPT dynamics for systems varying in shape and size. *Mol. Phys.* **1993**, *78*, 533–544.

[S13] Kumar, G.; Ohkubo, T.; Mukai, T.; Hono, K. Plasticity and microstructure of Zr–Cu–Al bulk metallic glasses. *Scripta Mater.* **2007**, *57*, 173–176.

[S14] Pauly, S.; Liu, G.; Gorantla, S.; Wang, G.; Kühn, U.; Kim, D. H.; Eckert, J. Criteria for tensile plasticity in Cu–Zr–Al bulk metallic glasses. *Acta Mater.* **2010**, *58*, 4883–4890.

[S15] Pauly, S.; Liu, G.; Wang, G.; Kühn, U.; Mattern, N.; Eckert, J. Microstructural heterogeneities governing the deformation of $Cu_{47.5}Zr_{47.5}Al_5$ bulk metallic glass composites. *Acta Mater.* **2009**, *57*, 5445–5453.

[S16] Barekar, N. S.; Pauly, S.; Kumar, R. B.; Kühn, U.; Dhindaw, B. K.; Eckert, J. Structure-property relations in bulk metallic Cu–Zr–Al alloys. *Mater. Sci. and Eng.* **2010**, *527*, 21–22.
